# Supplementary material for: Patch2Self: Denoising Diffusion MRI with Self-Supervised Learning
Source: arXiv:2011.01355 source file (2020-11-02)
Supplement: Supplementary file 1 [file supplementary.tex]

\section*{\LARGE{Appendix}}
\begin{appendix}
% PGSE Acquisition
Diffusion values at different gradient directions (each corresponding to a 3D volume) are used populate a $q$-space such that one diffusivity value corresponds to a particular gradient direction. From this $q$-space information, one can infer the signal structure within each voxel. To model this signal as a tensor (DTI), one typically measures six values in $q$-space to capture the 3D orientation information of the tensor. By fitting a tensor to each voxel, the spatial correlations between the tensors and their orientations can be used to reconstruct white-matter fibers (tracts). Gaussian assumption of the tensor model to hinders recovery of crossing fibers from the measured signal \cite{farquharson_tournier_calamante_fabinyi_schneider-kolsky_jackson_connelly_2013}. Hence, this $q$-space is often over-sampled (with high coverage and sampling density on the spherical grid) using a High Angular Resolution Diffusion Imaging (HARDI) \cite{descoteaux_2015} acquisition scheme. This paved way for Q-Ball imaging based techniques \cite{tuch_2004, descoteaux_angelino_fitzgibbons_deriche_2007, aganj_lenglet_sapiro_yacoub_ugurbil_harel_2009, tournier_calamante_connelly_2007} which employs spherical harmonic based signal decomposition to perform more accurate tractography with ability to represent crossing information.
\end{appendix}
